# Supplementary material for: Focus-Consistent Multi-Level Aggregation for Compositional Zero-Shot Learning
Source: arXiv:2408.17083 source file (2024-08-30)
Supplement: Supplementary file 1 [file 7.appendix.tex]

% \appendix

% \section{Datasets}

% \begin{table}
% \tablestyle{5pt}{1.0}
% \setlength\tabcolsep{3.4pt}
% \def\w{20pt} 
% \scalebox{0.85}{
%     \begin{tabular}{l|cccc|ccc|ccc}
%     &\multicolumn{4}{c}{\textbf{Train}} & \multicolumn{3}{|c|}{\textbf{Validate}} & \multicolumn{3}{c}{\textbf{Test}} \\
%     \textbf{Datatsets}&Attr. & Obj. & SP & I & SP & UP &I &SP&UP&I  \\
%     \shline
%     UT-Zappos~\shortcite{yu2014fine} & 16 & 12 & 83 & 23k & 15 &15 & 3k & 18 & 18 & 3k\\
%     C-GQA~\shortcite{naeem2021learning} & 413 & 674 & 6k & 27k & 1k &1k & 7k & 1k & 1k & 5k\\
%     Clothing16K~\shortcite{zhang2022learning}& 8 & 9 & 18 & 7k & 10 &10 & 5k & 9 & 8 & 3k\\
%     \end{tabular}
%     }
%     \caption{\textbf{The detailed statistics of the datasets.} (SP: \# seen compositions, UP: \# unseen compositions, I: \# images)}
% \label{table:dataset_info}
% % \vspace{-4mm}
% \end{table}

% UT-Zappos is a fine-grained dataset with images of shoes. The 12 kinds of shoes have 16 states in total, like \textit{canvas heels} and \textit{leather slippers}. C-GQA is a recently proposed dataset based on the Stanford GQA dataset~\cite{hudson2019gqa}.
% Compared to two other datasets, its images have abundant labels with hundreds of attributes and objects. Clothing16K is a dataset for multi-label classification on Kaggle. It consists of 16k images with 8 different clothing categories in 9 different colors. \cref{table:dataset_info} shows the detailed information of the three datasets. 

\section{Additional Ablation Study}
